# Supplementary material for: Repetita Iuvant: Data Repetition Allows SGD to Learn High-Dimensional Multi-Index Functions
Source: arXiv:2405.15459 source file (2025-02-10)
Supplement: Supplementary file 3 [file informal_saad_solla.tex]

\section{Informal derivation of the main results}
\label{sec:app:saad_solla}
\dots \, Maybe to fill with the derivation from informal saad e solla (without martingale control etc) of the dynamical behaviour of one-pass algorithms \dots 
